# Supplementary material for: Spin-Weighted Spherical Harmonics for Polarized Light Transport
Source: arXiv:2501.07582 source file (2024-12-29)
Supplement: Supplementary file 1 [file application2-supp.tex]

\section{Full Image Results for Polarimetric Radiance Fields}
Figure~\ref{fig:plenoxels_full} shows spin-2 SH-based radiance fields results without crop.

\begin{figure*}[t]
	\centering
	\footnotesize
	\setlength{\tabcolsep}{0pt}
	
	\begin{tabular}{cccccccccc}
		\centeredtab{\rotatebox[origin=c]{90}{P-Materials}} & 
		\centeredtab{\includegraphics[width=0.108\textwidth]{figs/plenoxels/materials/gt_0000_S0.jpg}} &
		\centeredtab{\includegraphics[width=0.108\textwidth]{figs/plenoxels/materials/gt_0000_S1_cm.jpg}} & 
		\centeredtab{\includegraphics[width=0.108\textwidth]{figs/plenoxels/materials/naive/pred_0000_S1_cm.jpg}} & 
		\centeredtab{\includegraphics[width=0.108\textwidth]{figs/plenoxels/materials/s2sh/pred_0000_S1_cm.jpg}} & 
		\centeredtab{\includegraphics[width=0.108\textwidth]{figs/plenoxels/materials/gt_0000_S2_cm.jpg}} & 
		\centeredtab{\includegraphics[width=0.108\textwidth]{figs/plenoxels/materials/naive/pred_0000_S2_cm.jpg}} & 
		\centeredtab{\includegraphics[width=0.108\textwidth]{figs/plenoxels/materials/s2sh/pred_0000_S2_cm.jpg}} &
		\centeredtab{\includegraphics[width=0.108\textwidth]{figs/plenoxels/materials/naive/err_0000.jpg}} & 
		\centeredtab{\includegraphics[width=0.108\textwidth]{figs/plenoxels/materials/s2sh/err_0000.jpg}}
		\\
		\centeredtab{\rotatebox[origin=c]{90}{P-Lego}} & 
		\centeredtab{\includegraphics[width=0.108\textwidth]{figs/plenoxels/lego/gt_0100_S0.jpg}} &
		\centeredtab{\includegraphics[width=0.108\textwidth]{figs/plenoxels/lego/gt_0100_S1_cm.jpg}} & 
		\centeredtab{\includegraphics[width=0.108\textwidth]{figs/plenoxels/lego/naive/pred_0100_S1_cm.jpg}} & 
		\centeredtab{\includegraphics[width=0.108\textwidth]{figs/plenoxels/lego/s2sh/pred_0100_S1_cm.jpg}} & 
		\centeredtab{\includegraphics[width=0.108\textwidth]{figs/plenoxels/lego/gt_0100_S2_cm.jpg}} & 
		\centeredtab{\includegraphics[width=0.108\textwidth]{figs/plenoxels/lego/naive/pred_0100_S2_cm.jpg}} & 
		\centeredtab{\includegraphics[width=0.108\textwidth]{figs/plenoxels/lego/s2sh/pred_0100_S2_cm.jpg}} &
		\centeredtab{\includegraphics[width=0.108\textwidth]{figs/plenoxels/lego/naive/err_0100.jpg}} & 
		\centeredtab{\includegraphics[width=0.108\textwidth]{figs/plenoxels/lego/s2sh/err_0100.jpg}}
		\\
		\centeredtab{\rotatebox[origin=c]{90}{P-Hotdog}} & 
		\centeredtab{\includegraphics[width=0.108\textwidth]{figs/plenoxels/hotdog/gt_0000_S0.jpg}} &
		\centeredtab{\includegraphics[width=0.108\textwidth]{figs/plenoxels/hotdog/gt_0000_S1_cm.jpg}} & 
		\centeredtab{\includegraphics[width=0.108\textwidth]{figs/plenoxels/hotdog/naive/pred_0000_S1_cm.jpg}} & 
		\centeredtab{\includegraphics[width=0.108\textwidth]{figs/plenoxels/hotdog/s2sh/pred_0000_S1_cm.jpg}} & 
		\centeredtab{\includegraphics[width=0.108\textwidth]{figs/plenoxels/hotdog/gt_0000_S2_cm.jpg}} & 
		\centeredtab{\includegraphics[width=0.108\textwidth]{figs/plenoxels/hotdog/naive/pred_0000_S2_cm.jpg}} & 
		\centeredtab{\includegraphics[width=0.108\textwidth]{figs/plenoxels/hotdog/s2sh/pred_0000_S2_cm.jpg}} &
		\centeredtab{\includegraphics[width=0.108\textwidth]{figs/plenoxels/hotdog/naive/err_0000.jpg}} & 
		\centeredtab{\includegraphics[width=0.108\textwidth]{figs/plenoxels/hotdog/s2sh/err_0000.jpg}}
		\\
        & RGB (GT) & $s_1$ (GT) & $s_1$ (Naïve) & $s_1$ (Spin-2 SH) & $s_2$ (GT) & $s_2$ (Naïve) & $s_2$ (Spin-2 SH) & Error (Naïve) & Error (Spin-2 SH) \\
	\end{tabular}
	\caption{
		\textbf{Full Image Results for Polarimetric Radiance Fields.}
	}
	\label{fig:plenoxels_full}
\end{figure*}
