# Supplementary material for: Spin-Weighted Spherical Harmonics for Polarized Light Transport
Source: arXiv:2501.07582 source file (2024-12-29)
Supplement: Supplementary file 2 [file application-s2l2-supp.tex]

\section{Application: S2L2 representation of single Stokes vectors}
\label{sec:app-s2l2}
\SHIN{TBATBA}

\begin{equation} \label{eq:app-s2l2-norm} %
	\begin{split}
		\sqrt{\sum_{m=-2}^2 \norm{\dvY_{2m}\left(\homega\right)}_\calS^2} &= \sqrt{\sum_{m=-2}^2 \abs{\sY{2m}\left(\theta,\phi\right)}^2} \\
		&=\frac18 \sqrt{\frac5\pi}\sqrt{6\sin^4 \theta + 4\sin^2\theta\left[\left(-1+\cos\theta\right)^2 + \left(-1-\cos\theta\right)^2\right] + \sum_{m=\pm 2}\left(1-m\cos\theta+\cos^2\theta\right)^2} \\
		&= \frac18 \sqrt{\frac5\pi}\sqrt{6\sin^4 \theta + 8\sin^2\theta + 8\sin^2\theta\cos^2\theta + 2 + 12 \cos^2 + 2\cos^4 \theta} =  \frac18 \sqrt{\frac5\pi}\sqrt{16} = \sqrt\frac{5}{4\pi}
	\end{split}
\end{equation}
